# Supplementary material for: Offset-corrected $\Delta$-Kohn-Sham scheme for the prediction of X-ray photoelectron spectra of molecules and solids
Source: arXiv:1511.06610 source file (2015-11-23)
Supplement: Supplementary file 1 [file SI.pdf]

# Supplemental Material for:
# Offset-corrected Δ-Kohn-Sham scheme for the prediction of X-ray photoelectron spectra of molecules and solids

Michael Walter*
*Freiburger Materialforschungszentrum, Universität Freiburg,*
*Stefan-Meier-Strae 21, D-79104 Freiburg, Germany and*
*Fraunhofer IWM, MikroTribologie Centrum µTC,*
*Wöhlerstrasse 11, D-79108 Freiburg, Germany*

Michael Moseler
*Freiburger Materialforschungszentrum, Universität Freiburg,*
*Stefan-Meier-Strae 21, D-79104 Freiburg, Germany*
*Fraunhofer IWM, MikroTribologie Centrum µTC,*
*Wöhlerstrasse 11, D-79108 Freiburg, Germany and*
*Physikalisches Institut, Universität Freiburg,*
*Herrmann-Herder-Strae 3, D-79104 Freiburg, Germany*

Lars Pastewka
*Fraunhofer IWM, MikroTribologie Centrum µTC,*
*Wöhlerstrasse 11, D-79108 Freiburg, Germany and*
*Karlsruher Institut für Technologie, Institut für Angewandte Materialien,*
*Engelbert-Arnold-Straße 4, D-76131 Karlsruhe, Germany*

## MOLECULES

The shorthand $Al(L_i)_3$, $i = 1 - 4$ was used for $L_1$=$CH_3COCHCOCH_3$, $L_2$=$CF_3COCHCOCH_3$, $L_3$=$CF_3COCHCOCF_3$, and $L_4$=$(CH_3)_3CCOCHCOC(CH_3)_3$ in fig. 2 of the main text. The values $E_B^{\mathrm{exp}}$ and $E_B^{\mathrm{calc}}$ shown in fig. 2 of the main text are reported in tables I-VIII below.

| molecule | $E_B^{\mathrm{exp}}$ | $E_B^{\mathrm{calc}}$ | $E_B^{\mathrm{calc}} - E_B^{\mathrm{exp}}$ |
|---|---|---|---|
| $(C^*H_3)_3PCH_2$ | 290.57 | 296.75 | 6.18 |
| $(CH_3)_3PC^*H_2$ | 288.00 | 294.24 | 6.24 |
| $CH_2O$ | 294.47 | 300.65 | 6.18 |
| $CH_3NH_2$ | 291.60 | 297.73 | 6.13 |
| $P(CH_3)_3$ | 290.30 | 296.40 | 6.10 |

continued

| | | | |
|---|---|---|---|
| $S(Si(CH_3)_3)_2$ | 289.79 | 295.90 | 6.11 |
| $CH_3SH$ | 291.41 | 297.69 | 6.28 |
| $Fe(CO)_5$ | 293.53±0.19 | 300.08 | 6.54∓0.19 |
| HCN | 293.40 | 299.66 | 6.26 |
| $CH_3OH$ | 292.51±0.29 | 298.57 | 6.06∓0.29 |
| $C_2H_4$ | 290.79±0.09 | 297.03 | 6.24∓0.09 |
| $(CH_3)_2SO$ | 291.24 | 297.33 | 6.09 |
| $C_6H_6$ | 290.33±0.09 | 296.49 | 6.16∓0.09 |
| $Si(CHi_3)_4$ | 289.78 | 295.88 | 6.10 |
| $Al(CF_3C^*OCHC^*OCF_3)_3$ | 294.06 | 299.90 | 5.84 |
| $Al(C^*F_3COCHCOC^*F_3)_3$ | 298.83 | 304.35 | 5.52 |
| $Al(CF_3COC^*HCOCF_3)_3$ | 291.30 | 297.41 | 6.11 |
| $S(CH_3)_2$ | 290.96±0.21 | 297.32 | 6.37∓0.21 |
| $Al((C^*H_3)_3C^*COCHCOC^*(C^*H_3)_3)_3$ | 289.97 | 296.46 | 6.49 |
| $Al((CH_3)_3CC^*OCHC^*OC(CH_3)_3)_3$ | 291.20 | 297.57 | 6.37 |
| $((CH_3)_2SiH)_2O$ | 289.93 | 296.03 | 6.10 |
| $(CH_3O)_2SO$ | 292.53 | 298.63 | 6.10 |
| $H_2Fe(CO)_4$ | 294.15 | 300.21 | 6.06 |
| $CH_3C^*N$ | 292.82±0.38 | 298.86 | 6.04∓0.38 |
| $C^*H_3CN$ | 293.04±0.06 | 298.82 | 5.78∓0.06 |
| $CH_3C^*OOH$ | 295.49±0.11 | 301.16 | 5.67∓0.11 |
| $C^*H_3COOH$ | 291.58±0.02 | 297.68 | 6.10∓0.02 |
| $CH_3SiHF_2$ | 290.80 | 297.13 | 6.33 |
| $Al(CH_3C^*OCHC^*OCH_3)_3$ | 292.07 | 298.00 | 5.93 |
| $Al(C^*H_3COCHCOC^*H_3)_3$ | 290.45 | 296.49 | 6.04 |
| $Al(CH_3COC^*HCOCH_3)_3$ | 289.38 | 295.42 | 6.04 |
| $CO_2$ | 297.66±0.09 | 303.41 | 5.75∓0.09 |
| $C_5H_5N$ | 290.90 | 297.46 | 6.56 |
| $CH_3SiH_3$ | 290.39±0.09 | 296.60 | 6.20∓0.09 |
| $Al(CF_3C^*OCHC^*OCH_3)_3$ | 293.14 | 298.95 | 5.81 |
| $Al(C^*F_3COCHCOCH_3)_3$ | 298.19 | 303.67 | 5.48 |
| $Al(CF_3COC^*HCOCH_3)_3$ | 290.44 | 296.40 | 5.96 |
| $Al(CF_3COCHCOC^*H_3)_3$ | 291.23 | 297.12 | 5.89 |
| pyrrole | 289.90 | 296.89 | 6.99 |
| CO | 296.15±0.09 | 302.47 | 6.32∓0.09 |
| $(CH_3O)_2SO_2$ | 293.18 | 299.11 | 5.93 |

continued

| | | | |
|---|---|---|---|
| $CH_3NO$ | 294.45 | 300.32 | 5.87 |

Table I: C(1s) core holes.

| molecule | $E_B^{exp}$ | $E_B^{calc}$ | $E_B^{calc} - E_B^{exp}$ |
|---|---|---|---|
| $CH_3NH_2$ | 405.14±0.03 | 412.16 | 7.02∓0.03 |
| N*NO | 408.65±0.12 | 415.45 | 6.79∓0.12 |
| NN*O | 412.56±0.07 | 419.21 | 6.65∓0.07 |
| NO | 410.48±0.32 | 417.78 | 7.30∓0.32 |
| HCN | 406.36±0.44 | 413.76 | 7.40∓0.44 |
| $C_3CN$ | 405.72±0.18 | 412.36 | 6.64∓0.18 |
| $H_2NNH_2$ | 406.10 | 413.02 | 6.92 |
| $CH_3CH_2CN$ | 405.36±0.06 | 412.11 | 6.75∓0.06 |
| $N_2$ | 409.94±0.04 | 416.82 | 6.88∓0.04 |
| $C_5H_5N$ | 404.82±0.12 | 411.65 | 6.83∓0.12 |
| $NH_3$ | 405.57±0.03 | 412.58 | 7.01∓0.03 |
| pyrrole | 406.00 | 413.21 | 7.21 |
| $CH_3NO$ | 406.39±0.06 | 413.52 | 7.14∓0.06 |

Table II. N(1s) core holes.

## SOLIDS

Experimental core level energies are reported for andalusite: Al(2p$_{3/2}$) [1, 2], sillimanite: O(1s) [1, 3, 4], AlN: Al(2p$_{3/2}$) [5–10], Si: Si(2p) [11–27], alpha-quartz: O(1s) [28–30], sillimanite: Si(2p) [1, 3, 4], andalusite: O(1s) [1, 2], CSi: Si(2p) [13, 31–40], Graphite: C(1s) [22, 39, 41–44], Diamond: C(1s) [45–48], AlN: N(1s) [5–7, 9], corundum: Al(2p$_{3/2}$) [8, 49–72], kyanite: O(1s) [1–3], sillimanite: Al(2p$_{3/2}$) [1, 3, 4], alpha-quartz: Si(2p) [28–30], CSi: C(1s) [31, 32, 34, 35, 38, 73, 74], kyanite: Al(2p$_{3/2}$) [1–3], Al: Al(2p$_{3/2}$) [5, 22, 55, 59, 67, 75–89], corundum: O(1s) [49–55, 58, 61, 62, 64, 68, 70–72, 88, 90–92], kyanite: Si(2p) [1–3], and andalusite: Si(2p) [1, 2]. Relative energies are reported for kyanite: O(1s)-Si(2p) [1–3], corundum: O(1s)-Al(2p$_{3/2}$) [53–55, 58, 61, 62, 64, 68, 70, 71], andalusite: Si(2p)-Al(2p$_{3/2}$) [1, 2], sillimanite: O(1s)-Si(2p) [1, 3, 4], CSi: C(1s)-Si(2p) [31, 32, 34], kyanite: Si(2p)-Al(2p$_{3/2}$) [1, 2], alpha-quartz: O(1s)-Si(2p) [28–30], AlN: N(1s)-Al(2p) [5–7, 9], sillimanite: Si(2p)-Al(2p$_{3/2}$) [1, 3, 4], and andalusite: O(1s)-Si(2p) [1, 2]. Calculated Al(2p) energies were obtained from Al(2p$_{3/2}$) energies using a spin-orbit splitting of 0.44 eV [93].

| molecule | $E_B^{exp}$ | $E_B^{calc}$ | $E_B^{calc} - E_B^{exp}$ |
|---|---|---|---|
| $CH_2O$ | 539.48±0.10 | 547.08 | 7.60∓0.10 |
| $P_4O_6$ | 539.25 | 546.47 | 7.22 |
| $OPCl_3$ | 538.04±0.06 | 545.53 | 7.49∓0.06 |
| $N_2O$ | 541.41±0.01 | 549.23 | 7.82∓0.01 |
| $OPF_3$ | 539.20±0.10 | 546.75 | 7.55∓0.10 |
| NO | 543.21±0.11 | 551.15 | 7.94∓0.11 |
| $Fe(CO)_5$ | 539.59±0.37 | 547.65 | 8.05∓0.37 |
| $CH_3OH$ | 539.08±0.12 | 546.71 | 7.63∓0.12 |
| $(CH_3)_2SO$ | 536.67 | 544.33 | 7.66 |
| $Al(L_3)_3$ | 538.91 | 546.52 | 7.61 |
| $Al(L_4)_3$ | 536.60 | 544.16 | 7.56 |
| $((CH_3)_2SiH)_2O$ | 537.32 | 544.80 | 7.48 |
| $O_2$ | 543.28±0.11 | 551.54 | 8.26∓0.11 |
| $H_2Fe(CO)_4$ | 540.17 | 547.72 | 7.55 |
| $H_2O$ | 539.86±0.07 | 547.50 | 7.65∓0.07 |
| $CH_3CO^*OH$ | 538.29 | 545.72 | 7.43 |
| $CH_3COO^*H$ | 540.00 | 547.67 | 7.67 |
| $Al(L_1)_3$ | 536.84 | 544.40 | 7.56 |
| $SO_2$ | 539.84 | 547.38 | 7.54 |
| $CO_2$ | 541.30±0.02 | 548.88 | 7.58∓0.02 |
| $(SiH_3)_2O$ | 538.60 | 545.76 | 7.16 |
| $Al(L_2)_3$ | 537.89 | 545.46 | 7.57 |
| CO | 542.43±0.14 | 550.14 | 7.71∓0.14 |
| $(CH_3O^*)_2SO_2$ | 539.03 | 547.37 | 8.34 |
| $(CH_3O)_2SO^*_2$ | 537.90 | 545.88 | 7.98 |
| $CH_3NO$ | 537.74 | 545.22 | 7.48 |

Table III. O(1s) core holes.

* Michael.Walter@fmf.uni-freiburg.de

[1] F. Ohuchi, S. Ghose, M. Engelhard, and D. Baer, Am Mineral **91**, 740 (2006).

[2] G. Biino and P. Groening, Eur J Mineral **10**, 423 (1998).

[3] P. Anderson and W. Swartz, Inorg Chem **13**, 2293 (1974).

[4] C. Wagner, J Vac Sci Technol **21**, 933 (1982).

| molecule | $E_B^{exp}$ | $E_B^{calc}$ | $E_B^{calc} - E_B^{exp}$ |
|---|---|---|---|
| $SiF_4$ | 694.70 | 703.09 | 8.39 |
| $OPF_3$ | 695.70±0.10 | 704.01 | 8.31∓0.10 |
| $SF_6$ | 695.04 | 703.41 | 8.37 |
| $Al(L_3)_3$ | 694.41 | 703.00 | 8.59 |
| $PF_5$ | 695.35±0.05 | 703.76 | 8.41∓0.05 |
| $PF_5$ | 694.15±0.05 | 702.75 | 8.60∓0.05 |
| $PF_3$ | 694.14±0.06 | 702.55 | 8.40∓0.06 |
| $SF_4$ | 695.26 | 703.53 | 8.27 |
| $SF_4$ | 692.88 | 701.41 | 8.53 |
| $Al(L_2)_3$ | 693.86 | 702.37 | 8.51 |

Table IV. F(1s) core holes.

| molecule | $E_B^{exp}$ | $E_B^{calc}$ | $E_B^{calc} - E_B^{exp}$ |
|---|---|---|---|
| $Al(L_1)_3$ | 79.50 | 80.21 | 0.71 |
| $Al(L_2)_3$ | 80.53 | 81.21 | 0.68 |
| $Al(L_3)_3$ | 81.61 | 82.27 | 0.66 |
| $Al(L_4)_3$ | 79.20 | 80.10 | 0.90 |

Table V. Al($2p_{3/2}$) core holes.


[5] J. Taylor and J. Rabalais, J. Chem. Phys. **75**, 1735 (1981).

[6] T. Hagio, A. Takase, and S. Umebayashi, Mater. Sci. Lett. **11**, 878 (1992).

[7] G. Martin, A. Botchkarev, A. Rockett, and H. Morkoc, Appl. Phys. Lett. **68**, 2541 (1996).

[8] G. McGuire, G. Schweitzer, and T. Carlson, Inorg. Chem. **12**, 2450 (1973).

[9] G. Martin, S. Strite, A. Botchkarev, A. Agarwal, A. Rockett, H. Morkoc, W. Lambrecht, and B. Segall, Appl. Phys. Lett. **65**, 610 (1994).

[10] J. Waldrop and R. Grant, Appl. Phys. Lett. **68**, 2879 (1996).

[11] J. Finster, E.-D. Klinkenberg, and Heeg, J. Vacuum **41**, 1586 (1990).

[12] R. Baptist, A. Pellissier, and G. Chauvet, Solid State Commun. **68**, 555 (1988).

[13] A. Tabata, S. Fujii, Y. Suzuoki, T. Mizutani, and M. Ieda, J. Phys. D. **23**, 316 (1990).

[14] G. Ingo, N. Zacchetti, S. D. della, and C. Coluzza, J. Vac. Sci. Technol. A **7**, 3048 (1989).

[15] R. Alfonsetti, L. Lozzi, M. Passacandanto, P. Picozzi, and S. Santucci, Appl. Surf. Sci. **70**, 222 (1993).

[16] M. Jeske, K. Jung, J. Schultze, M. Thonissen, and H. Munder, Surf. Interface Anal. **22**, 363 (1994).

[17] W. Chang, I. Bello, and W. Lau, J. Vac. Sci. Technol. A **11**, 1221 (1993).

[18] S. Morgan, R. Williams, and J. Mooney, Appl. Surf. Sci. **56**, 493 (1992).

[19] F. Sirotti, S. M. De, and G. Rossi, Phys. Rev. B **48**, 8299 (1993).

| molecule | $E_B^{\rm exp}$ | $E_B^{\rm calc}$ | $E_B^{\rm calc} - E_B^{\rm exp}$ |
|---|---|---|---|
| $SiF_4$ | 111.75±0.05 | 112.90 | 1.15∓0.05 |
| $Si(OC_2H_5)_4$ | 107.56 | 108.63 | 1.07 |
| $SiClH_3$ | 108.11 | 108.93 | 0.82 |
| $S(Si(CH_3)_3)_2$ | 106.57 | 107.04 | 0.47 |
| $(SiH_3)_2S$ | 107.45 | 108.13 | 0.68 |
| $Si(C_2H_3)_4$ | 106.03 | 106.81 | 0.78 |
| $SiH_4$ | 107.30±0.02 | 108.05 | 0.76∓0.02 |
| $Si(CHi_3)_4$ | 105.97±0.05 | 106.73 | 0.76∓0.05 |
| $((CH_3)_2SiH)_2O$ | 106.83 | 107.59 | 0.76 |
| $CH_3SiHF_2$ | 109.04 | 110.02 | 0.98 |
| $(SiH_3)_2O$ | 107.81 | 108.55 | 0.74 |
| $CH_3SiH_3$ | 106.88±0.07 | 107.62 | 0.74∓0.07 |
| $SiHCl_3$ | 109.44 | 110.27 | 0.83 |
| $(SiH_3)_2Se$ | 107.72 | 107.98 | 0.26 |
| $SiCl_4$ | 110.24±0.15 | 110.85 | 0.61∓0.15 |

Table VI. Si(2p) core holes.


[20] S. Chambers and V. Loebs, Phys. Rev. B **47**, 9513 (1993).

[21] T. Grehk, L. Johansson, S. Gray, M. Johansson, and A. Flodstrom, Phys. Rev. B **52**, 16593 (1995).

[22] C. Powell, J. Electron Spectrosc. Relat. Phenom. **185**, 1 (2012).

[23] E. Bruninx and T. Thijssen, Philips J. Res. **43**, 459 (1988).

[24] K. Magnusson, S. Wiklund, R. Dudde, and B. Reihl, Phys. Rev. B **44**, 5657 (1991).

[25] D. Rich, T. Miller, A. Samsavar, H. Lin, and T.-C. Chiang, Phys. Rev. B **37**, 10221 (1988).

[26] J. Gallego, R. Miranda, S. Molodtsov, C. Laubschat, and G. Kaindl, Surf. Sci. **239**, 203 (1990).

[27] R. Bringans, M. Olmstead, R. Uhrberg, and R. Bachrach, Phys. Rev. B **36**, 9569 (1987).

[28] V. P. Zakaznova-Herzog, H. W. Nesbitt, G. M. Bancroft, J. S. Tse, X. Gao, and W. Skinner, Phys. Rev. B **72** (2005).

[29] E. Grlich, J. Haber, A. Stoch, and J. Stoch, Journal of Solid State Chemistry **33**, 121 (1980).

[30] C. Tang, J. Zhu, Q. Zhou, J. Wei, R. Zhu, and H. He, J. Phys. Chem. C **118**, 26249 (2014).

[31] A. Galuska, J. Uht, and N. J. Marquez, Vac. Sci. Technol. A **6**, 110 (1988).

[32] M. Bozack, Surf. Sci. Spectra **3**, 82 (1994).

[33] S. Contarini, S. Howlett, C. Rizzo, and A. B. De, Appl. Surf. Sci. **51**, 177 (1991).

[34] M. Delplancke, J. Powers, G. Vandentop, M. Salmeron, and G. Somorjai, J. Vac. Sci. Technol. A **9**, 450 (1991).

[35] L. Johansson, F. Owman, and P. Martensson, Phys. Rev. B **53**, 13793 (1996).

[36] M. Hartley, J. Chiang, D. Hess, and D. Soane, Appl. Phys. Lett. **54**, 1510 (1989).

| molecule | $E_B^{\mathrm{exp}}$ | $E_B^{\mathrm{calc}}$ | $E_B^{\mathrm{calc}} - E_B^{\mathrm{exp}}$ |
|---|---|---|---|
| $(CH_3)_3PCH_2$ | 137.20 | 137.99 | 0.79 |
| $PH_3$ | 137.19±0.16 | 138.08 | 0.89∓0.16 |
| $P(C_2H_5)_3$ | 135.82 | 136.42 | 0.60 |
| $P_4O_6$ | 139.87 | 140.52 | 0.65 |
| $OPCl_3$ | 141.19±0.16 | 141.77 | 0.59∓0.16 |
| $P(CH_3)_3$ | 136.06±0.19 | 136.91 | 0.85∓0.19 |
| $OPF_3$ | 143.12±0.12 | 143.96 | 0.84∓0.12 |
| $SPCl_3$ | 140.89±0.26 | 141.28 | 0.39∓0.26 |
| $PF_5$ | 145.08±0.86 | 145.16 | 0.08∓0.86 |
| $PF_3$ | 141.92±0.13 | 142.66 | 0.75∓0.13 |
| $CH_3PH_2$ | 136.55 | 137.58 | 1.03 |
| $(CH_3O)_2PSCl$ | 140.13 | 140.67 | 0.54 |
| $PCli_3$ | 139.95±0.20 | 140.62 | 0.67∓0.20 |

Table VII. $P(2p_{3/2})$ core holes.

| molecule | $E_B^{\mathrm{exp}}$ | $E_B^{\mathrm{calc}}$ | $E_B^{\mathrm{calc}} - E_B^{\mathrm{exp}}$ |
|---|---|---|---|
| $S(Si(CH_3)_3)_2$ | 167.78 | 168.72 | 0.94 |
| $SF_6$ | 180.56±0.44 | 180.66 | 0.10∓0.44 |
| $CH_3SH$ | 169.39±0.12 | 170.78 | 1.39∓0.12 |
| $(SiH_3)_2S$ | 168.60 | 170.00 | 1.40 |
| $(CH_3)_2SO$ | 171.91 | 172.88 | 0.97 |
| $S(CH_3)_2$ | 169.09 | 170.27 | 1.18 |
| $SPCl_3$ | 169.03±0.16 | 170.11 | 1.08∓0.16 |
| $SH_2$ | 170.32±0.12 | 171.50 | 1.18∓0.12 |
| $(CH_3O)_2SO$ | 173.59 | 174.43 | 0.84 |
| $SF_4$ | 178.20 | 178.20 | 0.00 |
| $SO_2$ | 174.82±0.02 | 175.84 | 1.02∓0.02 |
| $(CH_3O)_2SO_2$ | 175.43 | 176.20 | 0.77 |

Table VIII. $S(2p_{3/2})$ core holes.

[37] L. Chen, T. Goto, T. Hirai, and T. Amano, J. Mater. Sci. Lett. **9**, 997 (1990).
[38] L. Muehlhoff, W. Choyke, M. Bozack, J. Yates, and Jr., J. Appl. Phys. **60**, 2842 (1986).
[39] K. Smith and K. Black, J. Vac. Sci. Technol. A **2**, 744 (1984).
[40] D. Niles, H. Hochst, G. Zajac, T. Fleisch, B.C., and M. J. Johnson, J. Vac. Sci. Technol. A **6**, 1584 (1988).

[41] Y. Xie and P. Sherwood, Surf. Sci. Spectra **1**, 367 (1992).

[42] G. Witek, M. Noeske, G. Mestl, S. Shaikhutdinov, and R. Behm, Catal. Lett. **37**, 35 (1996).

[43] Z. Bastl, Collect. Czech. Chem. Commun. **60**, 383 (1995).

[44] J. Keiser and R. Kleber, J. Appl. Phys. **9**, 315 (1976).

[45] R. Graupner, F. Maier, J. Ristein, L. Ley, and J. Ch., Phys. Rev. B **57**, 12397 (1998).

[46] T. Leung, W. Man, P. Lim, W. Chan, F. Gaspari, and S. Zukotynski, Journal of Non-Crystalline Solids **254**, 156 (1999).

[47] K. Sawa, J. du Plessis Materials Letters **58**, 1344 (2004).

[48] K. Yusaku, T. Jun, and M. Iwao, Diamond and Related Materials **13**, 93 (2004).

[49] J. T. Kloprogge, L. V. Duong, B. J. Wood, and R. L. Frost, Journal of Colloid and Interface Science **296**, 572 (2006).

[50] W. J. Gignac, R. S. Williams, and S. P. Kowalczyk, Phys. Rev. B **32**, 1237 (1985).

[51] A. Balzarotti and A. Bianconi, physica status solidi (b) **76**, 689 (1976).

[52] B. Strohmeier, Surf. Sci. Spectra **3**, 141 (1994).

[53] A. Dua, V. George, and R. Agarwala, Thin Solid Films **165**, 163 (1988).

[54] G. Ertl, R. Hierl, H. Knozinger, N. Thiele, and H. Urbach, Appl. Surf. Sci. **5**, 49 (1980).

[55] C. Wagner, D. Passoja, H. Hillery, T. Kinisky, H. Six, W. Jansen, and J. Taylor, J. Vac. Sci. Technol. **21**, 933 (1982).

[56] Ng, K. T., Hercules, and D. M., J. Phys. Chem. **80**, 2095 (1976).

[57] J. Lindsay, H. Rose, W. Swartz, P. Watts, and K. Rayburn, Appl. Spectrosc. **27**, 1 (1973).

[58] J. Kovacich and D. Lichtman, J. Electron Spectrosc. Relat. Phenom. **18**, 341 (1980).

[59] J. Klein and D. Hercules, J. Catal. **82**, 424 (1983).

[60] A. Hughes and B. Sexton, J. Electron Spectrosc. Relat. Phemon. **50**, c15 (1990).

[61] S. Andersson and M. Scurrell, J. Catal. **59**, 340 (1979).

[62] E. J. Paparazzo, Electron Spectrosc. Relat. Phemon. **43**, 97 (1987).

[63] Y. Okomoto, T. Imanaka, and S. Teranishi, J. Catal. **65**, 448 (1980).

[64] V. J. Nefedov, Electron Spectrosc. Relat. Phenom. **25**, 29 (1982).

[65] V. Nefedov, Salyn, Y.V., G. Leonhardt, and R. Scheibe, J. Electron Spectrosc. Relat. Phenom. **10**, 121 (1977).

[66] V. Nefedov, D. Gati, Dzhurinskii, B.F., N. Sergushin, and Y. Salyn, Zh. Neorg. Khimii **20**, 2307 (1975).

[67] A. Carley and M. Robers, Proc. Roy. Soc. Ser. A **363**, 403 (1978).

[68] B. Strohmeier and D. Hercules, J. Catal. **86**, 266 (1984).

[69] P. Breeze, H. Hartnagel, and P. Sherwood, J. Electrochem. Soc. **127**, 454 (1980).

[70] B. Strohmeier, D. Leyden, R. Field, and D. J. Hercules, Catal. **94**, 514 (1985).

[71] T. Barr, Appl. Surf. Sci. **15**, 1 (1983).

[72] N. Turner and A. Single, Surf. Interface Anal. **15**, 215 (1990).

[73] S. J. Kennou, Appl. Phys. **78**, 587 (1995).

[74] J. Waldrop, R. Grant, Y. Wang, and R. Davis, J. Appl. Phys. **72**, 4757 (1992).

[75] A. P. T. M. Van and J. Trooster, Phys. Rev. B **18**, 3872 (1978).

[76] R. Hauert, J. Patscheider, M. Tobler, and Zehringer, R. Surf. Sci. **292**, 121 (1993).

[77] M. Durrwachter, G. Indlekofer, H.-G. Boyen, P. Oelhafen, and D. J. Quitmann, Non-cryst. Solids **156**, 241 (1993).

[78] C. Hinnen, D. Imbert, J. Siffre, and P. Marcus, Appl. Surf. Sci. **78**, 219 (1994).

[79] K. Domen and T. Chuang, J. Chem. Phys. **90**, 3318 (1989).

[80] T. Sarapatka, J. Phys. Chem. **97**, 11274 (1993).

[81] A. Pashutski, A. Hoffman, and M. Folkman, Surf. Sci. **208**, L91 (1989).

[82] Y. Baba, T. Sasaki, and I. Takano, J. Vac. Sci. Technol. A **6**, 2945 (1988).

[83] P. Bagus, G. Pacchioni, and F. Parmigiani, Phys. Rev. B **43**, 5172 (1991).

[84] C. Wagner and J. Taylor, J. Electron Spectrosc. Relat. Phenom. **20**, 83 (1980).

[85] W. Schneider and C. Laubschat, Phys. Rev. B **20**, 4416 (1979).

[86] C. McConville, D. Seymour, D. Woodruff, and S. Bao, Surf. Sci. **188**, 1 (1987).

[87] L. Ley, F. McFeely, S. Kowalczyk, J. Jenkin, and D. Shirley, Phys. Rev. B **11**, 600 (1975).

[88] J. Taylor, J. Vac. Sci. Technol. **20**, 751 (1982).

[89] P. Steiner, H. Hoechst, and S. Hufner, Z. Physik B **30**, 129 (1978).

[90] J. Bonnelle, J. Grimblot, and A. J. D'huysser, Electron Spectrosc. Relat. Phenom. **7**, 151 (1975).

[91] K. Kishi and S. Ikeda, Bull. Chem. Soc. Jpn. **46**, 341 (1973).

[92] P. Zhdan, A. Shepelin, Z. Osipova, and V. Sokolovskii, J. Catal. **58**, 8 (1979).

[93] A. Agui, S. Shin, C. Wu, K. Shiba, and K. Inoue, Phys. Rev. B **59**, 10792 (1999).
